# Supplementary material for: Spatial Addressing of Qubits in a Dispersive Waveguide
Source: arXiv:2407.10617 source file (2024-07-15)

Qubit 1

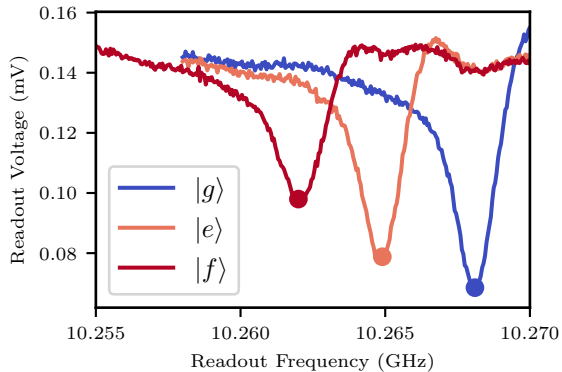

Qubit 2

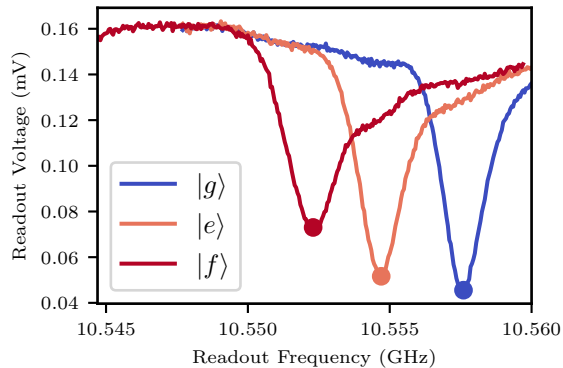

Qubit 1

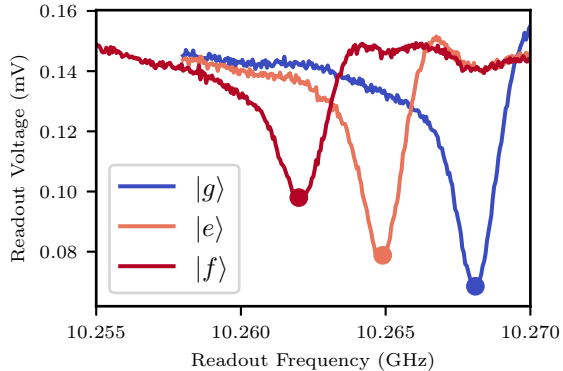

Qubit 2

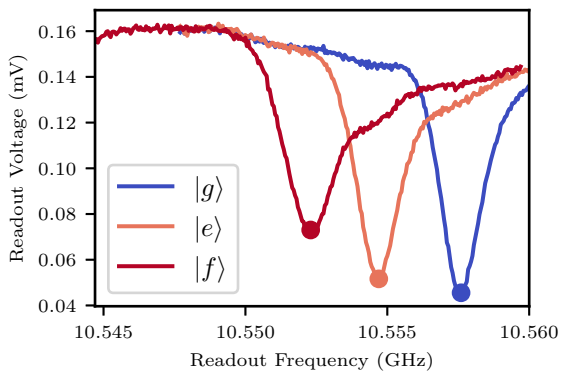

Supplement: Supplementary file 1 [file sup_disp_shifts_73.pdf]
